# Supplementary material for: Decoherence and Energy Relaxation in the Quantum-Classical Dynamics for Charge Transport in Organic Semiconducting Crystals: an Instantaneous Decoherence Correction Approach
Source: arXiv:1505.02234 source file (2015-05-09)
Supplement: Supplementary file 1 [file SupplementaryMaterial.pdf]

# Supplementary Material of Decoherence and Energy Relaxation in the Quantum-Classical Dynamics for Charge Transport in Organic Semiconducting Crystals: an Instantaneous Decoherence Correction Approach

Wei Si[1] and Chang-Qin Wu[1,2,a)]

[1)] *State Key Laboratory of Surface Physics and Department of Physics, Fudan University, Shanghai 200433, China*

[2)] *Collaborative Innovation Center of Advanced Microstructures, Fudan University, Shanghai 200433, China*

(Dated: 4 May 2015)

[a)]Email: cqw@fudan.edu.cn

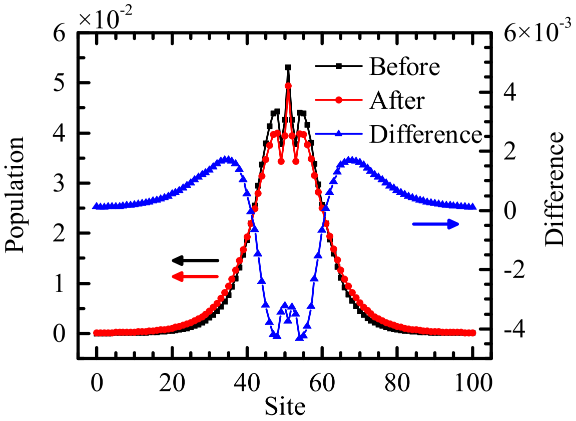


FIG. 1. Population distribution before (black square, $P^b$) and after (red circle, $P^a$) the decoherence correction by removing the phase coherence among different adiabatic states. The system starts from adiabatic states drawn from a Boltzmann distribution and is evolved after $50J/\hbar \approx 0.9$ps. The difference of the two distributions $P^a - P^b$ is also shown (blue triangle).

## I. ENHANCEMENT OF DIFFUSION

In Fig. 1, we show an example of the enhancement of diffusion by instantaneous decoherence corrections (IDC). The parameters are taken to be the typical set presented in the paper. The system is started in a random configuration of thermal equilibrium. The displacements and velocities are chosen from a Maxwell distribution and the electronic state chosen from a Boltzmann distribution. The evolution time is chosen to be $50J/\hbar \approx 0.9$ps. The decoherence correction is carried out by removing the phase coherence among different adiabatic states. It can be seen that the distribution after the decoherence correction ($P^a$) is wider than the distribution before the correction ($P^b$), which means the measurement-like operation enhances the diffusion. This can be seen more clearly from the difference of the two ($P^a - P^b$). The reason of this enhancement is analyzed in the paper

## II. LOCALIZATION LENGTH

In Fig. 2, we show the temperature dependence of the averaged localization length $\bar{l}_{\rm loc}$. The localization length is reflected by the inverse participation ratio (IPR), which is defined as

$$l_{\rm loc} = \frac{1}{\sum_j |\langle j\,|\psi\rangle\,|^4}. \tag{1}$$

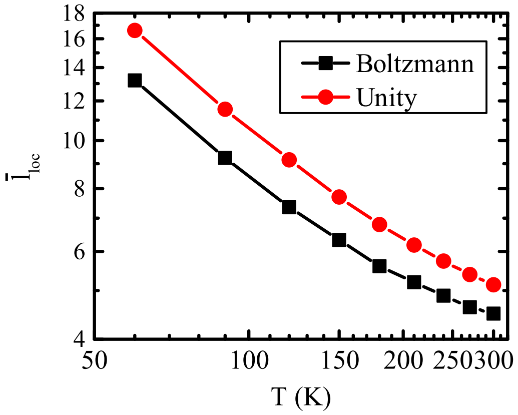


FIG. 2. Temperature dependence of averaged inverse participation ratio $\bar{l}_{\rm loc}$. The average is taken adiabatic states by both uniform and Boltzmann distribution.

where $j$ is the index for lattice sites and $\psi$ is the wave function. $\bar{l}_{\rm loc}$ is calculated by averaging the IPR of the adiabatic states by a certain distribution. Here, both the uniform distribution and the Boltzmann distribution are used. It can be seen that beyond 150 K, $\bar{l}_{\rm loc}$ show a deviation from a power-law dependence on temperature. As the diffusion constants with IDC is more closely related to the localization length of adiabatic states, this explains the similar deviations that is present there.

## III. POLARON EFFECTS

In Fig. 3, we show the evolution of the averaged absolute value of the displacements $\bar{|u|}(t)$. Two kinds of averaging procedure are used. The first one is the unweighted average, which is

$$\bar{|u|}_{\rm u}(t) = \frac{\sum_{s,j} |u_j(t)|}{N_L N_s}, \tag{2}$$

where $s$ is the index of realizations; $j$ is the index for lattice sites; $N_s$ is the number of samples and $N_L$ is the number of lattice sites. The second one is the weighted average, which is defined as

$$\bar{|u|}_{\rm w}(t) = \frac{\sum_{s,j} |\langle j|\psi^s(t)\rangle|^2 |u_j(t)|}{N_L N_s}, \tag{3}$$

where $\psi^s(t)$ is the wave function of the $s$-th realization at time $t$. The averaged potential energy of phonons is defined similarly. The unweighted average is

$$\bar{V}_{\rm ph,u}(t) = \frac{\sum_{s,j} m u_j^2}{2 N_L N_s}, \tag{4}$$

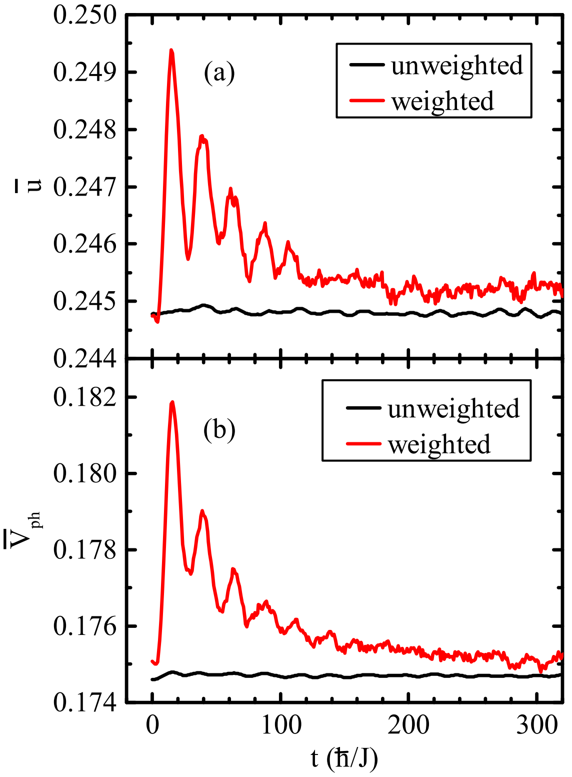


FIG. 3. Evolution of the unweighted and weighted average of the absolute value of the displacements (a) and phonon potential energy (b) with the Ehrenfest dynamics starting from randomly chosen adiabatic states with equal probability.

The weighted average is

$$\bar{V}_{\mathrm{ph,w}}(t) = \frac{\sum_{s,j} |\langle j|\psi^s(t)\rangle|^2 m u_j^2}{2N_L N_s}, \tag{5}$$

The weighted averaged reflect the effect of the presence of the carrier on the lattice by the Hellmann-Feynman force. The differences between the weighted and the unweighted average indicate a polaron effect in the system, which clearly the case in Fig. 2. With increasing time, the polaron effect is less pronounced due to the spread of the wave function and the effect of the Langevin heat bath.

## IV. ELECTRONIC ENERGY

The dependence of the averaged electronic energy $\bar{E}_{\mathrm{el}}$ at long times with respect to temperature is shown in Fig. 4, in which the Boltzmann value is also shown for comparison. The evolution time is taken to be $t = 10$ ps, when the $\bar{E}_{\mathrm{el}}$ with IDC-BM and IDC-MA have

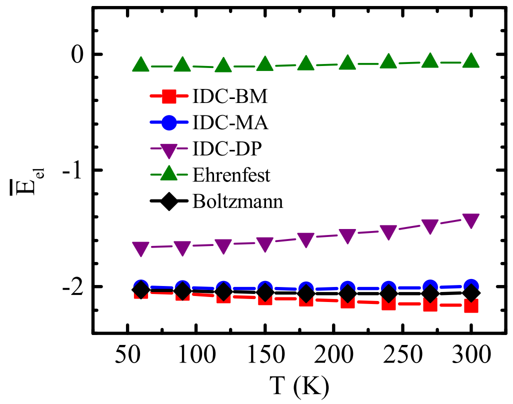


FIG. 4. Temperature dependence of the averaged electronic energy $\bar{E}_{\rm el}$ at long times with the IDC-BM (red square), IDC-MA (blue circle), IDC-DP (purple lower triangle) schemes and Ehrenfest (green diamond) dynamics. The Boltzmann value (black diamond) is shown for comparison. The values with the Ehrenfest dynamics and IDC-DP are taken at 10 ps.

converged. The $\bar{E}_{\rm el}$ with Ehrenfest dynamics and IDC-DP converge much more slowly and the values at $t = 10$ ps are shown for reference. It can be seen that both IDC-BM and IDC-MA give final energies that are close to the Boltzmann value in the whole temperature range concerned. The values with IDC-BM are slightly smaller than the Boltzmann ones, while the values with IDC-MA are slightly larger than the Boltzmann ones. However, the values with IDC-DP and the Ehrenfest dynamics deviate clearly from the Boltzmann value.

## V. POPULATION AND PROBABILITY DISTRIBUTION

In Fig. 3 (a) and (b), we show the population distribution and the probability distribution from the dynamics with IDC after evolving the system for 10 ps. The whole energy regime is taken for clarity.

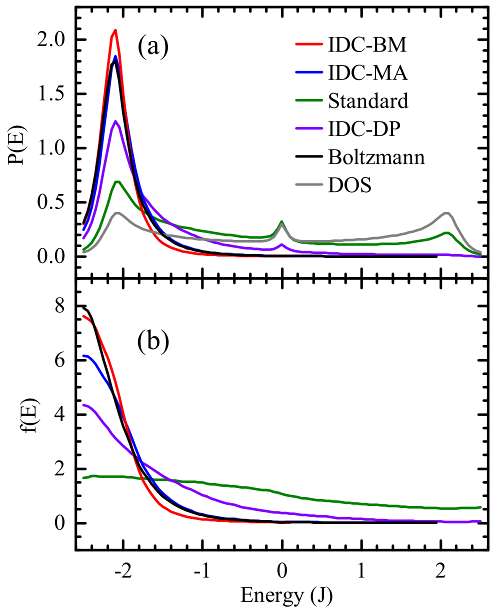


FIG. 5. (a) Population distribution after evolution of 10 ps from an initial state with randomly chosen adiabatic states with equal probability. The results from the IDC-BM, IDC-MA, IDC-DP and Ehrenfest dynamics are shown. The results from the Boltzmann distribution and the density of states (DOS) are shown for guide. (b) Probability distribution after evolution of 10 ps from an initial state with randomly chosen adiabatic states with equal probability. The results from the IDC-BM, IDC-MA, Troisi's standard and IDC-DP methods are shown. The results from the Boltzmann distribution are shown for guide.
